# Supplementary material for: CobBO: Coordinate Backoff Bayesian Optimization with Two-Stage Kernels
Source: arXiv:2101.05147 source file (2022-04-19)
Supplement: Supplementary file 1 [file appendix_Arxiv.tex]

\onecolumn
\icmltitle{
CobBO: Coordinate Backoff Bayesian Optimization - 
Supplementary Materials}
\appendix

 \section{Default hyper-parameter configuration}
\label{sec:defalt_conf}
Table~\ref{table:hyperparameters} contains the default configuration of CobBO, which is used to test all the experiments in this paper. 
\begin{table}[h!]
\centering
\begin{tabular}{ |c|c|c| } 
\hline
Hyperparameter & Description & Default Value \\
\hline \hline
$\Theta$ & The threshold for the number of consecutive fails $q_t$ before changing $V_t$ & $60$ if $T>2000$ else $30$\\ 
\hline
$\alpha$ & Increase multiplicative ratio for the coordinate distribution update & $2.0$\\ 
\hline
$\beta$ & Decay multiplicative ratio for the coordinate distribution update  & $1.1$\\ 
\hline
$p$ & Probability for selecting coordinates with the largest $\pi_t$ values & $0.3$\\ 
\hline
$\kappa_S$ & \makecell{The threshold for the virtual clock value $K_t$ \\before shrinking the coarse trust region $\Omega_{S}$} & $30$\\ 
\hline
$\kappa_F$ & \makecell{The threshold for the number of consecutive fails $q_t$ before \\shrinking the fine trust region $\Omega_{F}$ on the fast time scale} & $6$\\ 
%\hline
%$\tau_S$ & The number of consecutive fails $q_t$ in the coarse trust region $\Omega_{S}$ & $8$\\ 
\hline
$\tau_F$ & The number of consecutive fails $q_t$ in the fine trust region $\Omega_{F}$  & $6$\\ 
\hline
$\delta$ & The relative improvement threshold governing the virtual clock update rule & $0.1$\\ 
\hline
& Gussian process kernel & Matern 5/2 \\
\hline
\end{tabular}
\caption{CobBO's hyperparameters configuration for all of the experiments}
\label{table:hyperparameters}
\end{table}

\section{Implementation} %IMPLEMENTATION}
The proposed CobBO algorithm is implemented in Python~3. \\
An implementation of CobBO is available at: \url{https://github.com/Alibaba-MIIL/CobBO}.

\section{Further ablation of escaping local optima}
CobBO is described in Algorithm~1, where Line~8 is about escaping local maxima by changing the pivot point $V_t$ when the number of consecutive fails exceeds a threshold, i.e., $q_t>\Theta$.
In this case, we decrease the observed function value at $V_{t}$ and set $V_{t+1}$ as a selected sub-optimal random point in $\mathcal{X}_t$. Specifically, we randomly sample $5$ points in $\mathcal{X}_t$ with their values above the median and pick the one furthest away from $V_{t}$. 

%  In order to escape stagnant local optima, CobBO has two methods. The first method is to change $V_t$, as described in Section~2 of the paper. The threshold $\Theta_1$ for the number of consecutive fails $q_t$ before changing $V_t$ is set to $70$ if the total
%  trial budget is larger than $2000$ otherwise $\Theta_1=35$. 
%  The second method is decrease the function values around the stagnant local optima. Specifically, when the number of consecutive trials $\Theta_2$ that fail to improve the optimization process, e.g., $\Theta_2=50$ if the total
%  trial budget is larger than $2000$ otherwise $\Theta_2=25$, we temporary decrease the function values around the best point observed so far.  By doing so, the Gaussian process regression could encourage to explore other potentially more promising areas.

We use the experiments on Levy and Ackley functions of 100 dimensions, as described in section~3.2 to compute the fraction of queries that improve
 the already observed maximal points due to changing~$V_t$ according to Line~8.  
 
 \begin{table}[h!]
\centering
\begin{tabular}{ |c|c|c| } 
\hline
Problem & Average \# improved queries & Average \# improved queries due to escaping\\
\hline \hline
Ackley & 228 & 15.3 \\
\hline
Levy & 155 & 3\\
\hline
\end{tabular}
\caption{The number of improved queries due to escaping local maxima}
\label{table:escaping}
\end{table}

We observe that optimizing the Levy function yields very few queries that improve the maximal points by changing the pivot point, while optimizing the Ackley function can benefit more from that.  

\section{Forming trust regions on two time scales}
CobBO alternates between the two trust regions according to a duty cycle determined by $\kappa_F$ and $\tau_F$ as specified by Algorithm~1 and Table~\ref{table:hyperparameters}.  %~\ref{alg:trust_region}.
The formation of trust regions is triggered when a virtual clock $K_t$, expressing the progress of the optimization, reaches certain thresholds.
Specifically, the virtual clock evolves as following
  \begin{align*}
    K_{t+1}=
    \begin{cases}
		K_t + 1	 & \text{if } \Delta_t \leq 0 \\
	   % \gamma_t(\Delta_t, ||x_t - x_{t-1}||) \cdot K_t & \text{if } 0 < \Delta_t \leq \delta \\
	    \gamma_t(\Delta_t, x_t, x_{t-1}) \cdot K_t & \text{if } 0 < \Delta_t \leq \delta \\
		0	 & \text{if } \Delta_t > \delta\\
	 \end{cases} 
 \end{align*}
which is described in equation~(3) in the main body of the paper.
%  where $\Delta_t = \frac{M_t - M_{t-1}}{\left|M_{t-1}\right|}$ is the relative improvement and for example, 

%  \begin{align*}
% 	 \gamma_t(\Delta, x_t, x_{t-1}) = \left(1-\frac{\Delta}{\delta}\right) \cdot \left(1 - \frac{||x_t - x_{t-1}||}{\sqrt{|C_t|}} \right).
%  \end{align*}

\begin{algorithm}[tbh]\vspace{0.0mm}
    \label{alg:trust_region}
% 	\SetAlgoLined
    % \textbf{Input}: Current virtual Clock $K_t$\\
    \textbf{Parameters}: \\
    \hspace{0.5cm} Slow/fast thresholds $\kappa_{S/F}$ respectively\\
    \hspace{0.5cm} Fast duty cycle $\tau_{F}$\\
    % Current observed value $y_t$ \\
    % Previous best value $M_{t-1}$ \\
    % Consecutive fails to improve $q_t$ \\
    \textbf{Init}: $\Omega_{0}, \tilde{\Omega}_{0} \leftarrow \Omega$ \\
    \uIf{$y_t > M_{t-1}$} {
        $\tilde{\Omega}_{t} \leftarrow$ Double $\tilde{\Omega}_{t-1}$ around $V_t$ \\
        $\Omega_{t} \leftarrow \tilde{\Omega}_{t}$ [$\tilde{\Omega}_{t}$ is the trust region formed on the slow time scale]
    }
    \uElseIf{$K_t==\kappa_S$}{
        $\tilde{\Omega}_{t} \leftarrow$ Halve $\tilde{\Omega}_{t}$ around $V_t$ \\
        $\Omega_{t} \leftarrow \tilde{\Omega}_{t}$\\
        Reset $K_t = 0$
    }
    \uElse{
        $\tilde{\Omega}_t \leftarrow \tilde{\Omega}_{t-1}$\\
        \uIf{$mod\left(K_t, \kappa_F+\tau_F\right)== \kappa_F-1$}{
         $\Omega_{t} \leftarrow$ Halve $\Omega_{t-1}$ around $V_t$
     }
     
     \uElseIf{$mod\left(K_t, \kappa_F+\tau_F\right)==  \kappa_F+\tau_F -1$}{
         $\Omega_{t} \leftarrow \tilde{\Omega}_{t}$}
     \uElse{$\Omega_{t} \leftarrow \Omega_{t-1}$}
    }

    %\uIf{
    %     $\tilde{\Omega}_t \leftarrow \Omega_{F_t}$
    %}
    % $\tilde{\Omega}_{t} \leftarrow \Omega_{S_t} \textbf{ If } mod\left(q_t, \tau_S+\tau_F\right) < \tau_S\textbf{ Else } \Omega_{F_t}\$
    % \IfThenElse {$mod\left(q_t, \tau_S+\tau_F\right) < \tau_S$}% If ...
    %   {$\Omega_{S_t}$}% ...then...
    %   {$\Omega_{F_t}$}% ...else...
      
    \textbf{Output}: Trust Region $\Omega_{t}$
	\caption{FormTrustRegions($K_t$,$y_t$,$M_{t-1}$)}
% 	\caption{FormTrustRegionsPolicy($K_t$, $\kappa_S$, $\kappa_F$, $\tau_S$, $\tau_F$, $y_t$, $M_{t-1}$, $q_t$)}
\end{algorithm}
\setlength{\textfloatsep}{0pt}

% The threshold $\kappa_S$ is not necessarily a constant. To adapt to different optimization problems, we choose $\kappa_S$ to depend on $\eta_t$ the number of times $K_t$ has consecutively reached $\kappa_S$. 
% When $\eta_t$ crosses a certain threshold,
% %that depends on the query budget $T$ and the problem dimension $D$,
% CobBO assumes being trapped in a local optimum~\cite{qin2017,bull2011,snoek2012}. 
% In this case, it 
% %randomly samples a point  reduces the function values in $\mathcal{H}_t$ within a small region around $V_t$, and 
% sets $V_{t+1}$ as
%  one of the already queried top points in $\mathcal{X}_t$ far away from $V_t$, and repeats the entire process
%  by starting with the full domain $\Omega$
%  and $\eta_{t+1}=0$.
 In addition, when the number of queried points exceeds a threshold, e.g., $70\%$ of the query budget, we shrink the total space~$\Omega$ every time when the fraction of the queried points increases by $10\%$.

\section{Additional experiments}
We provide more experiments for demonstrating the performance of CobBO. Confidence intervals ($95\%$) are computed by repeating $30$ and $10$ independent experiments for the medium-sized functions and the $200$-dimensional functions, respectively.

   \begin{figure}[bht]\vspace{-0mm}
   \centering
   \includegraphics[width=1.0\columnwidth,height=!]{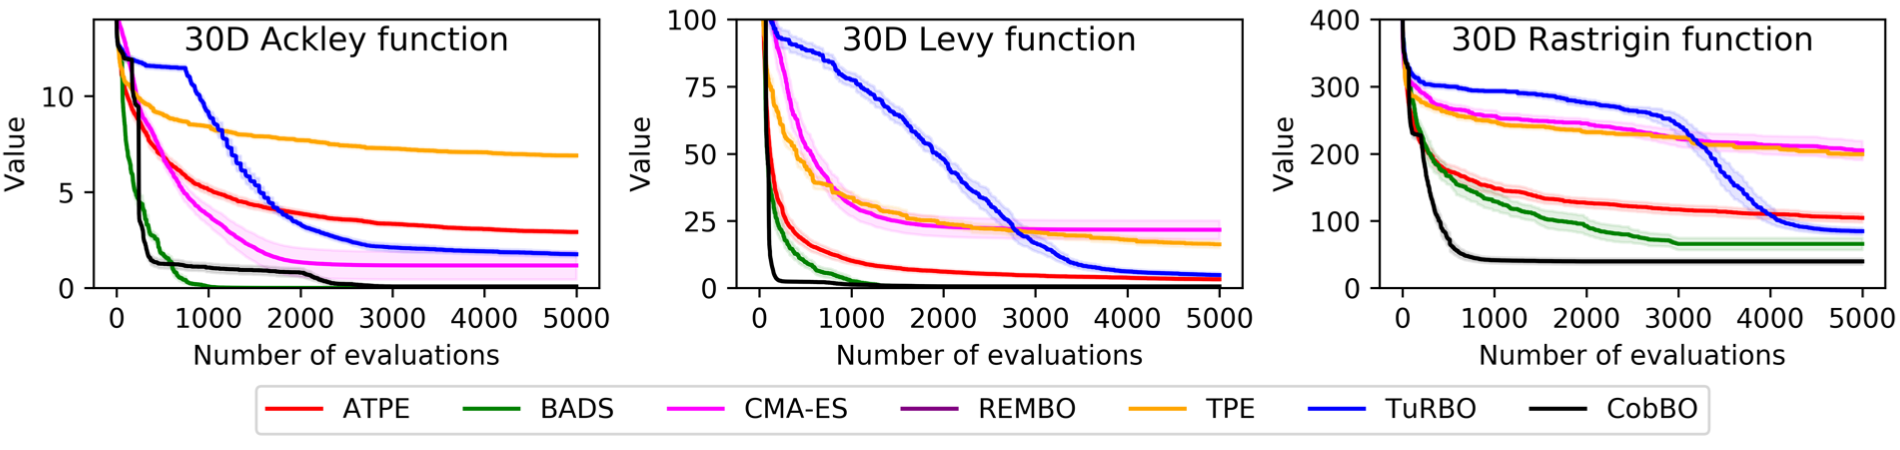}\vspace{-3mm}
   \caption{Performance over medium dimensional problems: Ackley (left), Levy (middle) and Rastrigin (right)} 
   \label{fig:30D-tests}
 \end{figure}
\textbf{Medium-sized synthetic black-box functions (minimization):}
We test three synthetic functions ($30$ dimensions), including Ackley on $[-5, 10]^{30}$, Levy $[-5, 10]^{30}$, and Rastrigin on $[-3, 4]^{30}$. In addition, 
we add experiments for an additive function of $36$ dimensions, defined as  $f_{36}(x)=\rm{Ackley}(x_1) + \rm{Levy}(x_2) + \rm{Rastrigin}(x_3) + \rm{Hartmann}(x_4)$, where the first three terms express the same functions over the same domains specified in Section~3.1 of this paper, with the Hartmann function over $[0, 1]^{6}$. 
TuRBO is configured identically the same as in Section~3.1, with a batch size of 10 and 5 trust regions with 10 initial points each. The other algorithms use 20 initial points.
The results are shown in Fig.~\ref{fig:30D-tests} and~\ref{fig:additive-36D}, where CobBO shows competitive or better performance compared to all of the methods tested across all of these problems.
 \begin{figure}[htb]\vspace{-0mm}
   \centering
   \includegraphics[width=0.7\columnwidth,height=!]{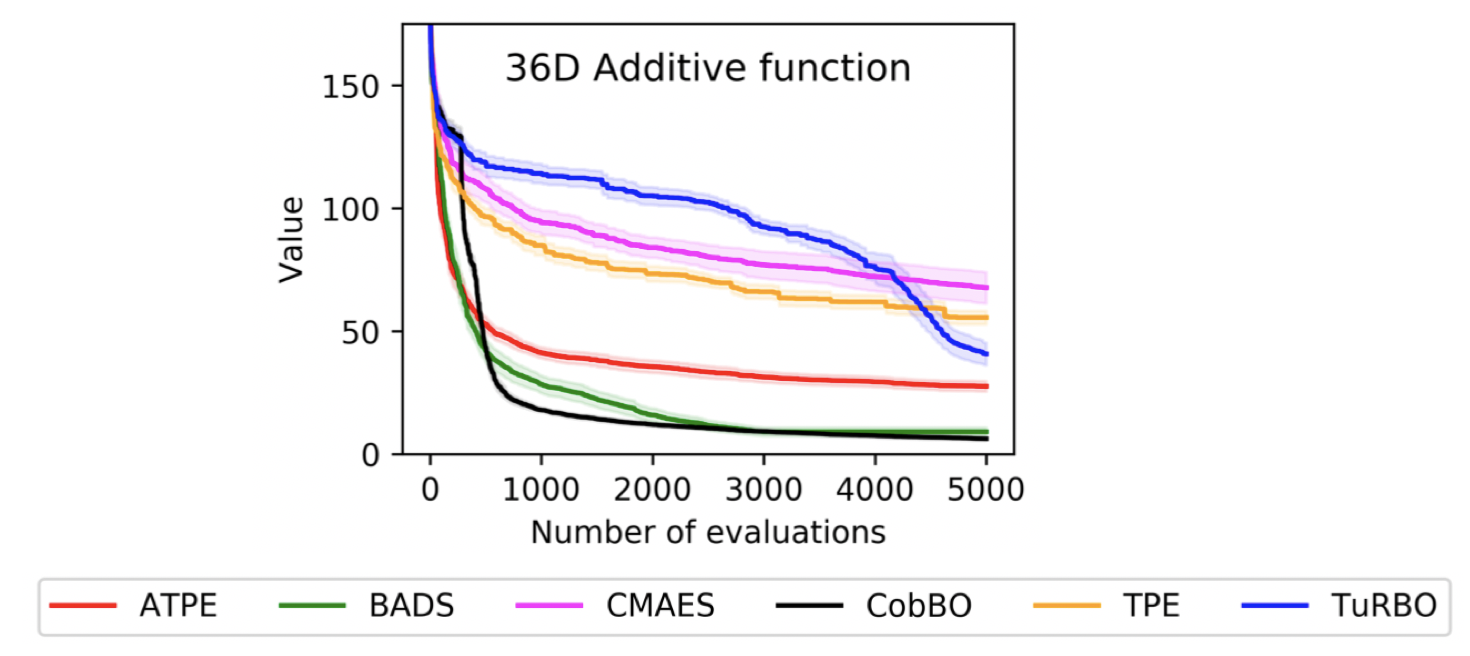}\vspace{1mm}
   \caption{Performance over an additive function of 36 dimensions}\vspace{5mm}
   \label{fig:additive-36D}
 \end{figure}

\textbf{The 200-dimensional Levy and Ackley functions (minimization):}
We minimize the Levy and Ackley functions over $[-5, 10]^{200}$ with $500$ initial points. 
TuRBO is configured with $15$ trust regions and a batch size of $100$.
These two problems are challenging and have no redundant dimensions. 
 For Levy, in Fig.~\ref{fig:200d} (left), CobBO reaches $100.0$ within $2,000$ trials, while CMA-ES and TuRBO 
 obtain $200.0$ after $8,000$ trials. TPE cannot find a comparable solution within $10,000$ trials in this case. 
 For Ackley, in Fig.~\ref{fig:200d} (right), CobBO reaches the best solution among all of the algorithms tested. 
 The appealing trial complexity of CobBO suggests that it can be applied in a hybrid method, e.g., used in the first stage of the query process combined with gradient estimation methods or CMA-ES.
%  Note that the variance for the Levy function across $10$ independent experiments is very small, as shown in Fig.~\ref{fig:200d-zoomin}. 

  \begin{figure}[htb]\vspace{-0mm}
   \centering
   \includegraphics[width=0.8\columnwidth,height=!]{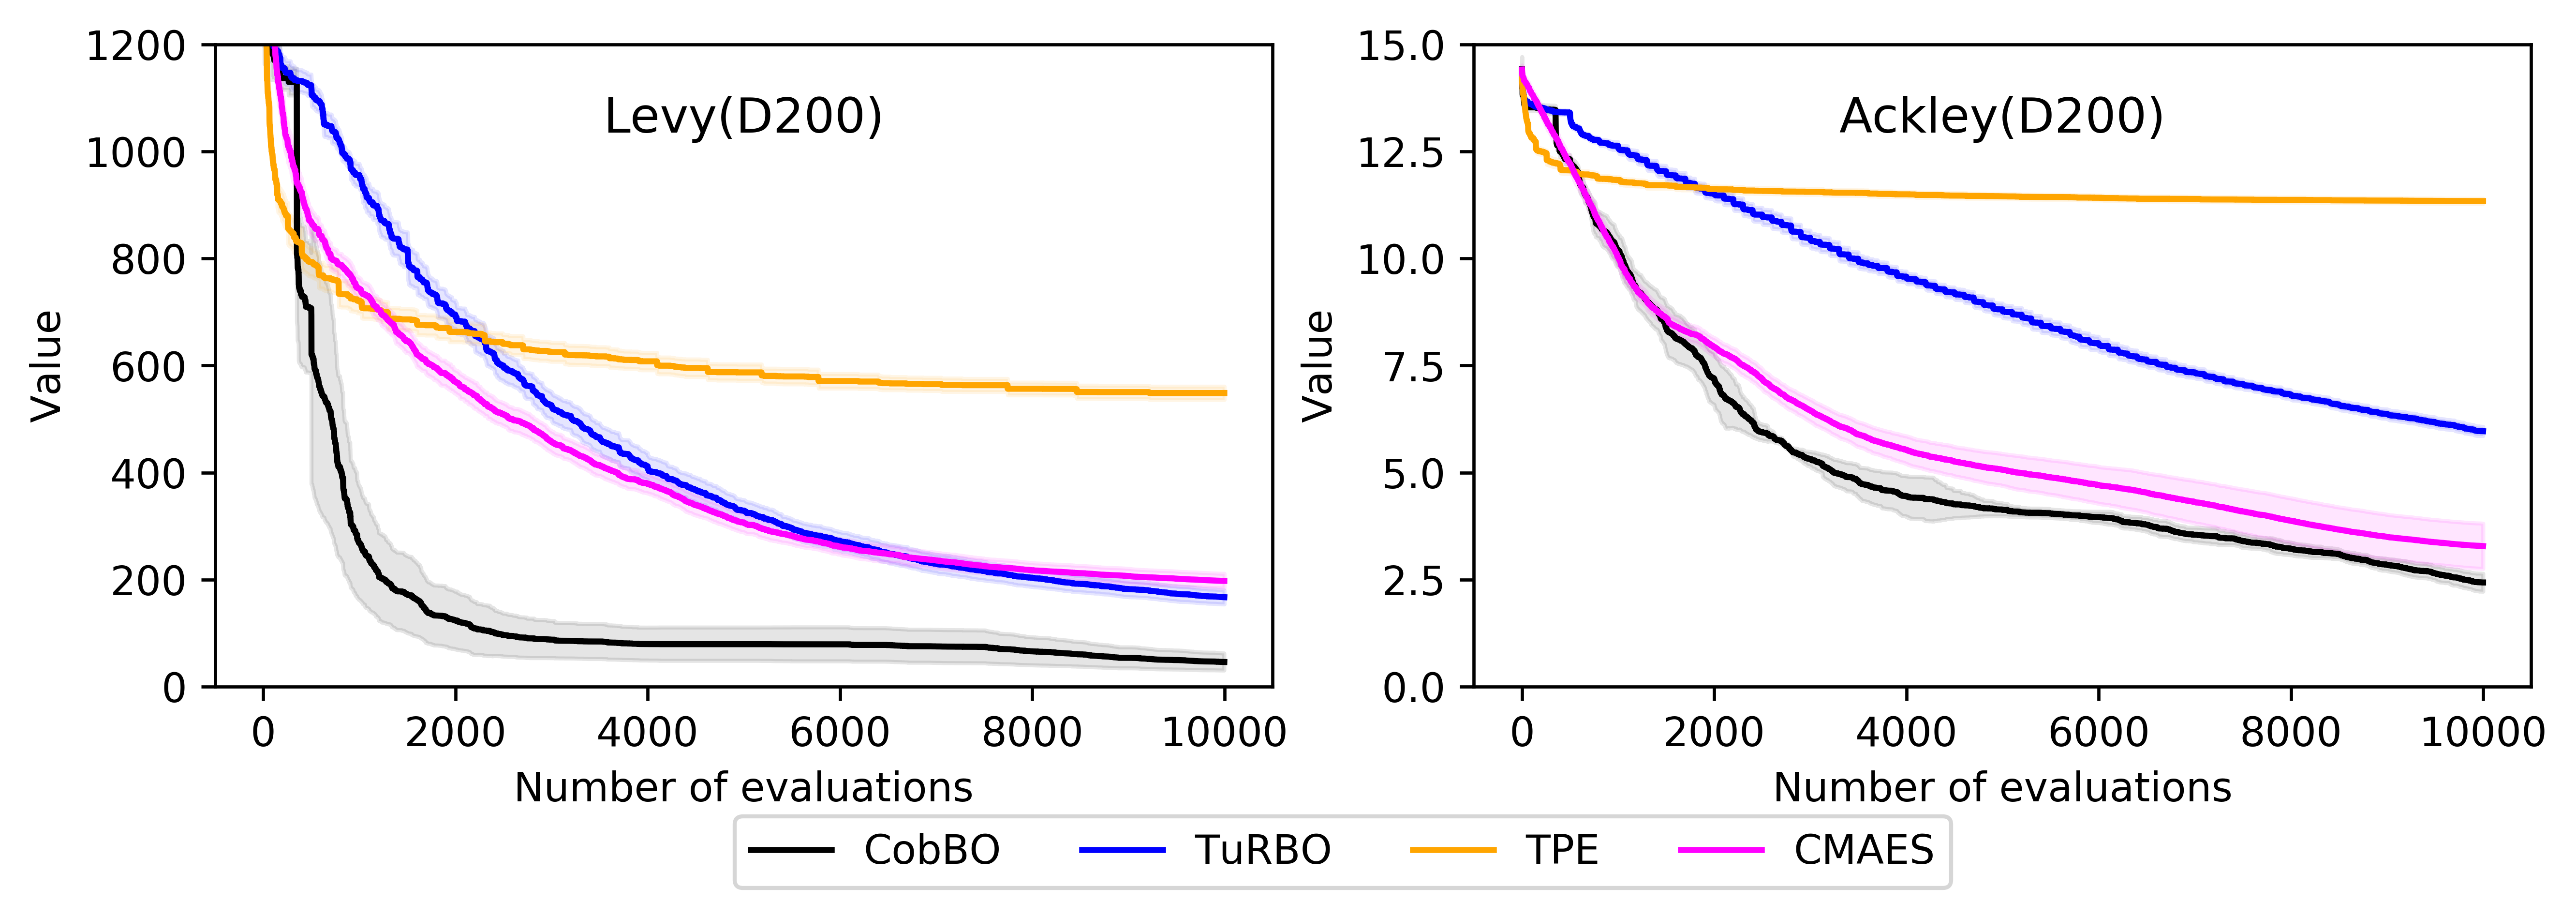}\vspace{-4mm}
   \caption{Performance over high dimensional synthetic problems: Levy (left) and Ackley (right)}\vspace{-0mm}
   \label{fig:200d}
 \end{figure}
% \vspace{-3mm}
%  \begin{figure}[htb]
%   \centering
%   \includegraphics[width=0.5\columnwidth,height=!]{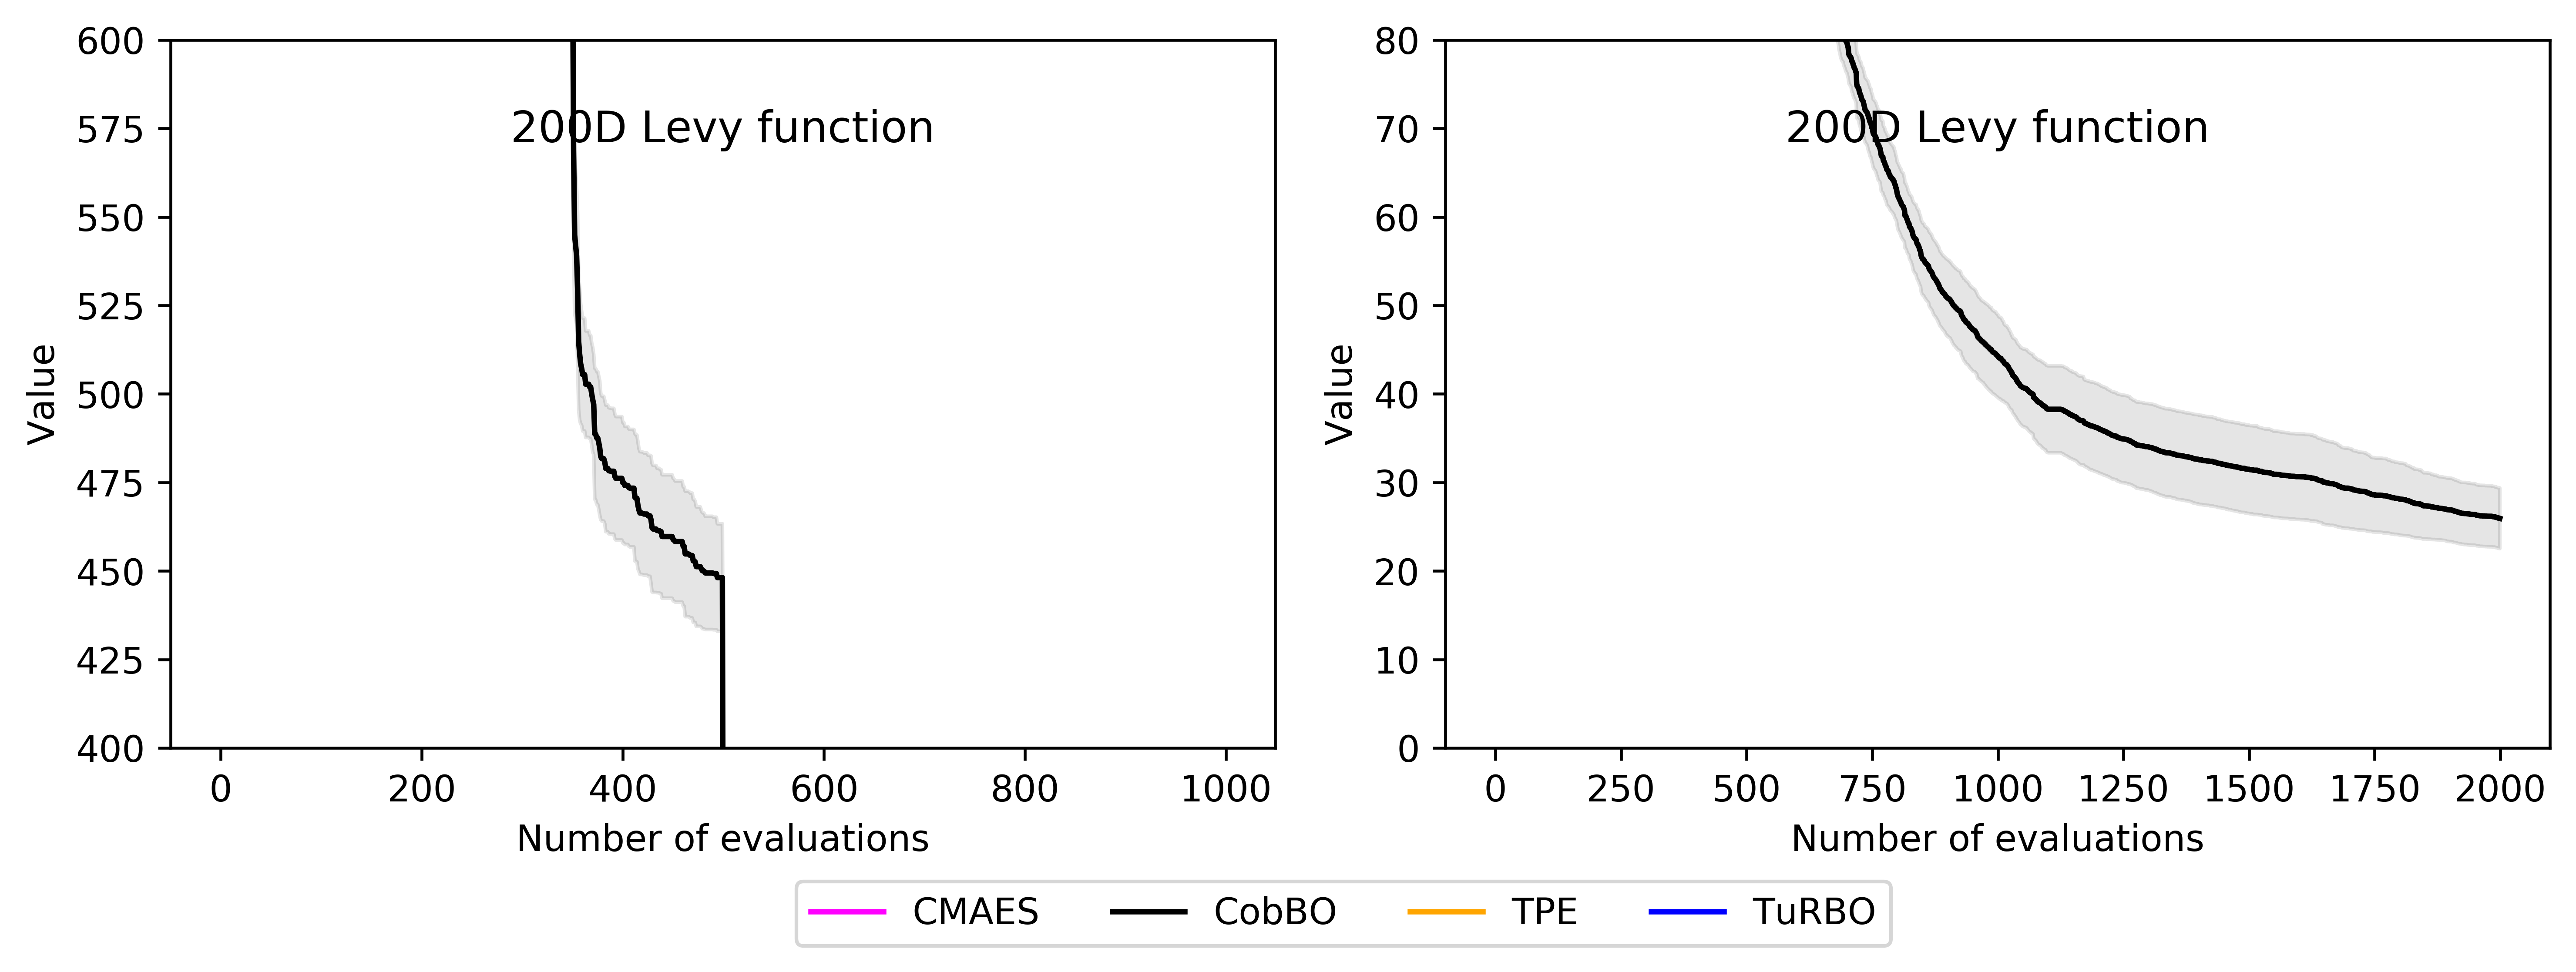}\vspace{-4mm}
%   \caption{A closer look at the performance over the high dimensional synthetic Levy problem}\vspace{-0mm}
%   \label{fig:200d-zoomin}
%  \end{figure}
