# Supplementary material for: CobBO: Coordinate Backoff Bayesian Optimization with Two-Stage Kernels
Source: arXiv:2101.05147 source file (2022-04-19)
Supplement: Supplementary file 3 [file parameters_table.tex]

\begin{table}[h]
\begin{center}
\begin{tabular}{ |c|c|c| } 
\hline
Parameter & Description & Default Value \\
\hline \hline
$\Theta$ & The threshold for the number of consecutive fails $q_t$ before changing $V_t$ & $70$\\ 
\hline
$\alpha$ & Increase multiplicative ratio for the coordinate distribution update & $1.2$\\ 
\hline
$\beta$ & Decay multiplicative ratio for the coordinate distribution update  & $1.8$\\ 
\hline
$p$ & Probability for selecting coordinates with the largest $\pi_t$ values & $0.3$\\ 
\hline
$\kappa_S$ & \makecell{The slow threshold for the virtual clock value $K_t$ \\before shrinking the coarse trust region $\Omega_{S}$} & $30$\\ 
\hline
$\kappa_F$ & \makecell{The fast threshold for the number of consecutive fails $q_t$ \\before shrinking the fine trust region $\Omega_{F}$} & $6$\\ 
\hline
$\tau_S$ & The number of consecutive fails $q_t$ in the course trust region $\Omega_{S}$ & $24$\\ 
\hline
$\tau_F$ & The number of consecutive fails $q_t$ in the fine trust region $\Omega_{F}$  & $6$\\ 
\hline
$\delta$ & The relative improvement threshold governing the virtual clock update rule & $0.1$\\ 
\hline
& Gussian process kernel & Matern 5/2 \\
\hline
\end{tabular}
\caption{CobBO's hyperparameters configuration for all of the experiments}
\label{table:hyperparameters}
\end{center}
\end{table}
